# Supplementary material for: Zero-shot Object-Centric Instruction Following: Integrating Foundation Models with Traditional Navigation
Source: arXiv:2411.07848 source file (2025-05-07)
Supplement: Supplementary file 1 [file appendix.tex]

\section{Supplementary Material}
\label{sec:appendix}

\subsection{Preliminaries: Factor Graphs}
\label{sec:prelim_factor}

Factor graphs~\cite{koller2009probabilistic} are probabilistic graphical models~\footnote{\url{https://gtsam.org/tutorials/intro.html}} and are widely used to model complex problems in Robotics.
A factor graph is a bipartite graph consisting of variables, representing unknown random variables and factors, representing constraints on the variables. The factors are local in nature such that they are dependent on a subset of the entire set of variables. The entire factor graph then captures the global function of variables as a product of multiple local functions~\cite{dellaert2017factor}. Factor graphs can be used to model different estimation problems in Robotics, such as Simultaneous Localization and Mapping (SLAM). In our work, we specifically focus on pose graph optimization along with landmark measurements.

Formally, a factor graph is represented as $F = (U, V, E)$ where $U$ is a set of factors $\phi_i$, V is the set of variables $x_j$, and E are the edges $e_{ij}$ between the factors and variables nodes. 
$N(\phi_i)$ is the set of variable nodes adjacent to the factor $\phi_i$ and $\pose_i$ is an assignment to this set. Then the factor graph $F$ can be defined as the factorization of a global function $\phi(X)$ as:
\begin{equation}
\label{eq:factors}
    \phi(X) = \prod_i{\phi(X_i)}
\end{equation}

\mypara{Pose Graph.}
A factor graph can be used to represent a pose graph where the variables represent the robot poses ($\pose_i$), including position and orientation and the factors ($f_i$) are the odometry measurements between the poses. The pose $x_1$ is the initial pose which is considered a prior. Optimizing the factor graph then means finding the best set of poses that satisfy the odometry constraints as closely as possible.

\mypara{Pose Graph with Landmarks.}
A factor graph can also contain the observed landmarks ($\obslandmark_i$) as a second type of variables in addition to robot poses ($\pose_i$). The poses are connected by factors representing odometry measurement. A landmark and a pose are connected by a factor $fl_{i}$ representing the observation measurement. 
An example is shown in \Cref{fig:prelim_landmark_slam}, where each small black node is a factor and connected to the variables it depends on. 

\begin{figure}[ht]
\centering
\begin{tikzpicture}[node distance={15mm}, thick, main/.style = {draw, circle}] 
\node[main] (1) [fill = black] {};
\node[main] (2) [right of=1] {$x_1$};
\node[main] (3) [right of=2] [fill = black] {};
\node[main] (4) [right of=3] {$x_2$};
\node[main] (5) [right of=4] [fill = black] {};
\node[main] (6) [right of=5] {$x_3$};
% \node[main] (7) [right of=6] [fill = black] {};
\node[main] (8) [above of=4] [fill = black] {};
\node[main] (9) [above of=8] {$l_1$};
\node[main] (10) [above of=3] [fill = black] {};
\node[main] (11) [above of=6] [fill = black] {};
\node[main] (12) [above of=11] {$l_2$};
\draw (1) -- (2);
\draw (2) -- (3);
\draw (3) -- (4);
\draw (4) -- (5);
\draw (5) -- (6);
% \draw (6) -- (7);
\draw (4) -- (8);
\draw (8) -- (9);
\draw (2) -- (10);
\draw (9) -- (10);
\draw (6) -- (11);
\draw (11) -- (12);
\end{tikzpicture} 
\caption{Landmark-based SLAM}
\label{fig:prelim_landmark_slam}
\end{figure}

\mypara{Pose Graph Optimization in SLAM.}
Pose Graph Optimization~\cite{dellaert2017factor} in SLAM improves the predicted robot poses, while it moves through an environment. This is done by minimizing the error between the predicted and the observed poses by taking into consideration the relationships and constraints between the poses and the observed landmarks. 
Following \Cref{eq:factors}, we can write the example factor graph from \Cref{fig:prelim_landmark_slam} in terms of the following factorization:
\begin{equation}
\label{eq:factor_graph_example}
    \phi(l_1,l_2,x_1,x_2,x_3) = 
            \phi(x_1) \phi(x_2,x_1) \phi(x_3,x_2)
            \phi(x_1,l_1)\phi(x_2,l_1)
            \phi(x_3,l_2)
\end{equation}

It can be shown that maximum a posteriori (MAP) inference for SLAM with a Gaussian noise model is equivalent to solving a nonlinear least-squares problem (for details refer to \cite{dellaert2017factor}). 
Assuming all factors follow the following form with Gaussian noise:
\begin{equation}
\label{eq:factor_graph_gaussian}
    \phi(X_i) \propto 
            \exp \{
                -\frac{1}{2} ||h_i(X_i) - z_i||^2_{\sum_i}
            \},
\end{equation}
MAP inference is equivalent to minimizing a sum of nonlinear least-squares:
\begin{equation}
\label{eq:factor_graph_map}
    X^{MAP} = argmin_x \sum_i ||h_i(X_i) - z_i||^2_{\sum_i}
\end{equation}
where $h(.)$ is a measurement prediction function and the measurement from a given pose x to a landmark l is modeled by $z = h(x, l) + \eta$. Here $\eta$ is a noise drawn from a zero-mean Gaussian density. The measurement functions $h(.)$ is non-linear in the Robotics applications, since the odometry factors are non-linear consisting of the robot orientation.
Nonlinear optimization methods such as the Levenberg-Marquardt (LM) algorithm can then be applied to converge to the global minimum in \Cref{eq:factor_graph_map} through linear approximations.

% A way to estimate the robot poses is through maximum a posteriori (MAP). It maximizes the posterior density $p(X|Z)$ of the states $X=\{x_1,x_2,...\}$ given the measurements $Z=\{z_1,z_2,...\}$.

% \begin{equation}
% \label{eq:map_basic}
%     X^{MAP} = argmax_x~p(X|Z)
%             = argmax_x~\frac{p(Z|X)p(X)}{p(Z)}
% \end{equation}

% \Cref{eq:map_basic} can be written as \Cref{eq:map_refined}, by ignoring the normalization factor p(Z), since the measurements Z are given and p(Z) do not contribute to the maximization.

% \begin{equation}
% \label{eq:map_refined}
%     X^{MAP} = argmax_x~l(X;Z)p(X)
% \end{equation}

% Here, l(X;Z) is the likelihood of the states X given Z, which is proportional to $p(Z|X)$.
